# Supplementary material for: (Almost Full) EFX for Three (and More) Types of Agents
Source: arXiv:2301.10632 source file (2025-01-02)
Supplement: Supplementary file 1 [file appendix.tex]

\appendix

\begin{center}
    \Large{Technical Appendix}    
\end{center}
